# Supplementary material for: Parameter Estimation-Based States Reconstruction of Uncertain Linear Systems with Overparameterization and Unknown Additive Perturbations
Source: arXiv:2308.10289 ancillary file (2024-03-13)
Supplement: Supplementary file 1 [file supp.pdf]

# Supplement to "Parameter Estimation-Based States Reconstruction of Uncertain Linear Systems with Overparameterization and Unknown Additive Perturbations"

Anton Glushchenko, *Member, IEEE* and Konstantin Lastochkin

**Abstract**

This article is a supplementary material for "Parameter Estimation-Based States Reconstruction of Uncertain Linear Systems with Overparameterization and Unknown Additive Perturbations" by the same authors. It provides proofs of Proposition 1, Proposition 2, Lemma, describes the derivation of the equations (27) and (35) and validates the hypothesis 1.

## I. Proof of Proposition 1 in the Manuscript

***Proposition 1.*** *There exists sufficiently large $t_\epsilon \geq t_0$ such that for all $t \geq t_\epsilon$ the following claims hold:*

$$\overline{q}\left(t\right) = f^{\mathrm{T}}F\left(t\right) + y\left(t\right) - C_0^{\mathrm{T}}z\left(t\right) = \overline{\varphi}_e^{\mathrm{T}}\left(t\right)\eta_e\left(\psi\right), \tag{8}$$

$$\begin{gathered}\xi\left(t\right) = z\left(t\right) + \Omega\left(t\right)\psi_a\left(\theta\right) + P\left(t\right)\psi_b\left(\theta\right) + \\ +\mathcal{O}_e^{-1}\mathcal{O}_\Gamma\left(\Gamma\right)\left(F\left(t\right) - N\left(t\right)\psi_a\left(\theta\right) - H\left(t\right)\psi_b\left(\theta\right)\right),\end{gathered} \tag{9}$$

*where*

$$\begin{gathered}\overline{\varphi}_e\left(t\right) = \begin{bmatrix}\Omega^{\mathrm{T}}C_0 + N^{\mathrm{T}}f \\ P^{\mathrm{T}}C_0 + H^{\mathrm{T}}f \\ F \\ vec\left(N\right) \\ vec\left(H\right)\end{bmatrix}, \eta_e\left(\psi\right) = \begin{bmatrix}\psi_a \\ \psi_b \\ \Gamma \\ -\psi_a\otimes\Gamma \\ -\psi_b\otimes\Gamma\end{bmatrix}, \\ \psi = \begin{bmatrix}\psi_a^{\mathrm{T}}\left(\theta\right) & \psi_b^{\mathrm{T}}\left(\theta\right) & \Gamma^{\mathrm{T}}\end{bmatrix}^{\mathrm{T}},\end{gathered} \tag{10}$$

$$\mathcal{O}_e = \begin{bmatrix}C_0^{\mathrm{T}} \\ C_0^{\mathrm{T}}A_K \\ \vdots \\ C_0^{\mathrm{T}}A_K^{n-1}\end{bmatrix}, \mathcal{O}_\Gamma\left(\Gamma\right) = \begin{bmatrix}\left(\Gamma - f\right)^{\mathrm{T}} \\ \left(\Gamma - f\right)^{\mathrm{T}}A_\Gamma \\ \vdots \\ \left(\Gamma - f\right)^{\mathrm{T}}A_\Gamma^{n-1}\end{bmatrix}, \tag{11}$$

$$\begin{gathered}\dot{z}\left(t\right) = A_Kz\left(t\right) + Ky\left(t\right), z\left(t_0\right) = 0_n, \\ \dot{P}\left(t\right) = A_KP\left(t\right) + I_nu\left(t\right), P\left(t_0\right) = 0_{n\times n}, \\ \dot{\Omega}\left(t\right) = A_K\Omega\left(t\right) + I_ny\left(t\right), \Omega\left(t_0\right) = 0_{n\times n}, \\ \dot{F}\left(t\right) = A_fF\left(t\right) + \\ +e_n\left[y\left(t\right) - C_0^{\mathrm{T}}z\left(t\right)\right], F\left(t_0\right) = 0_n, \\ \dot{H}\left(t\right) = A_fH\left(t\right) + e_nC_0^{\mathrm{T}}P\left(t\right), H\left(t_0\right) = 0_{n\times n}, \\ \dot{N}\left(t\right) = A_fN\left(t\right) + e_nC_0^{\mathrm{T}}\Omega\left(t\right), N\left(t_0\right) = 0_{n\times n},\end{gathered} \tag{12}$$

*Here the matrices $A_K$, $A_\Gamma$, $A_f$ have the following structure:*

$$\begin{gathered}A_K = \begin{bmatrix}-K & \begin{matrix}I_{n-1} \\ 0_{1\times(n-1)}\end{matrix}\end{bmatrix}, A_\Gamma = \begin{bmatrix}\begin{matrix}0_{(n-1)\times 1} & I_{n-1}\end{matrix} \\ \Gamma^{\mathrm{T}}\end{bmatrix}, \\ A_f = \begin{bmatrix}\begin{matrix}0_{(n-1)\times 1} & I_{n-1}\end{matrix} \\ f^{\mathrm{T}}\end{bmatrix},\end{gathered}$$

*while it holds that $\sigma\left(A_\Gamma\right) := \sigma\left(\mathcal{A}_\delta\left(\rho\right)\right) \cup 0_{n-n_\delta}$.*

*Proof:* Define the error:

$$e\left(t\right) = \xi\left(t\right) - z\left(t\right) - \Omega\left(t\right)\psi_a\left(\theta\right) - P\left(t\right)\psi_b\left(\theta\right). \tag{S1}$$

Equation (S1) is differentiated with respect to time to obtain:

$$\begin{gathered}\dot{e}\left(t\right) = A_0\xi\left(t\right) + \psi_a\left(\theta\right)y\left(t\right) + \psi_b\left(\theta\right)u\left(t\right) + e_n\psi_d\left(\theta\right)\delta\left(t\right) - A_Kz\left(t\right) - Ky\left(t\right) - \\ -\left(A_K\Omega\left(t\right) + I_ny\left(t\right)\right)\psi_a\left(\theta\right) - \left(A_KP\left(t\right) + I_nu\left(t\right)\right)\psi_b\left(\theta\right) = \\ = A_0\xi\left(t\right) - A_Kz\left(t\right) - Ky\left(t\right) - A_K\Omega\left(t\right)\psi_a\left(\theta\right) - A_KP\left(t\right)\psi_b\left(\theta\right) + e_n\psi_d\left(\theta\right)\delta\left(t\right) = \\ = A_Ke\left(t\right) + e_n\psi_d\left(\theta\right)\delta\left(t\right).\end{gathered} \tag{S2}$$

Financial support is in part provided by the Grants Council of the President of the Russian Federation (MD-1787.2022.4).
A. Glushchenko is with V.A. Trapeznikov Institute of Control Sciences of Russian Academy of Sciences, Moscow, Russia aiglush@ipu.ru
K. Lastochkin is with V.A. Trapeznikov Institute of Control Sciences of Russian Academy of Sciences, Moscow, Russia lastconst@ipu.ru

Equation (S2) is combined with (4) to write a cascade linear system:

$$\begin{array}{l} \dot{x}_\delta(t) = \mathcal{A}_\delta(\rho)\, x_\delta(t)\,, \\ \dot{e}(t) = A_K e(t) + \psi_d(\theta)\, e_n h_\delta^{\mathrm{T}} x_\delta(t)\,. \end{array} \tag{S3}$$

Define the error *a novo*:

$$\epsilon(t) = e(t) - \Pi(\rho)\, x_\delta(t)\,, \tag{S4}$$

where the matrix $\Pi(\rho)$ is unknown, but it is a solution of the Sylvester equation:

$$\Pi(\rho)\, \mathcal{A}_\delta(\rho) = A_K \Pi(\rho) + \psi_d(\theta)\, e_n h_\delta^{\mathrm{T}}, \tag{S5}$$

which has a unique solution as $\left(h_\delta^{\mathrm{T}}, \mathcal{A}_\delta(\rho)\right)$ is observable, $\left(A_K, \psi_d(\theta)\, e_n\right)$ is controllable and $\sigma\{A_K\} \cap \sigma\{\Pi(\rho)\} = 0$.

Equation (S4) is differentiated with respect to time to write:

$$\begin{array}{l} \dot{\epsilon}(t) = A_K e(t) + \psi_d(\theta)\, e_n h_\delta^{\mathrm{T}} x_\delta(t) - \Pi(\rho)\, \mathcal{A}_\delta(\rho)\, x_\delta(t) = \\ = A_K e(t) + \psi_d(\theta)\, e_n h_\delta^{\mathrm{T}} x_\delta(t) - A_K \Pi(\rho)\, x_\delta(t) - \psi_d(\theta)\, e_n h_\delta^{\mathrm{T}} x_\delta(t) = A_K \epsilon(t)\,, \end{array} \tag{S6}$$

from which:

$$e(t) = \epsilon(t) + \Pi(\rho)\, x_\delta(t)\,, \tag{S7}$$

and, therefore, taking into consideration that $A_K$ is a Hurwitz matrix, it holds for a sufficiently large $t_\epsilon \geq t_0$ that:

$$e(t) = \Pi(\rho)\, x_\delta(t)\,. \tag{S8}$$

Combining (S1) and (S8), it is obtained that:

$$\begin{array}{c} \xi(t) - z(t) - \Omega(t)\, \psi_a(\theta) - P(t)\, \psi_b(\theta) = \Pi(\rho)\, x_\delta(t) \\ \Downarrow \\ y(t) - C_0^{\mathrm{T}} z(t) = C_0^{\mathrm{T}} \Omega(t)\, \psi_a(\theta) + C_0^{\mathrm{T}} P(t)\, \psi_b(\theta) + C_0^{\mathrm{T}} \Pi(\rho)\, x_\delta(t)\,. \end{array} \tag{S9}$$

The summand $C_0^{\mathrm{T}} \Pi(\rho)\, x_\delta(t)$ needs to be parametrized as a multiplication of unknown parameters and measurable signals. To do that, let the following filter be introduced:

$$\begin{array}{l} \dot{\Psi}(t) = A_f \Psi(t) + e_n \left[C_0^{\mathrm{T}} \Pi(\rho)\, x_\delta(t) + C_0^{\mathrm{T}}(t)\right] = \\ = A_f \Psi(t) + e_n \left[y(t) - C_0^{\mathrm{T}} z(t) - C_0^{\mathrm{T}} \Omega(t)\, \psi_a(\theta) - C_0^{\mathrm{T}} P(t)\, \psi_b(\theta)\right]. \end{array} \tag{S10}$$

Using the supplementary lemma from [12], it holds for the derivative $\dot{\Psi}(t)$ that:

$$\dot{\Psi}(t) = A_\Gamma \Psi(t) + e_n \varepsilon(t)\,, \tag{S11}$$

where

$$A_\Gamma = \begin{bmatrix} 0_{(n-1)\times 1} & I_{n-1} \\ \multicolumn{2}{c}{\Gamma^{\mathrm{T}}} \end{bmatrix},\ A_f = \begin{bmatrix} 0_{(n-1)\times 1} & I_{n-1} \\ \multicolumn{2}{c}{f^{\mathrm{T}}} \end{bmatrix},$$

and $\varepsilon(t)$ stands for an exponentially decaying signal.

Owing to the structures of $A_\Gamma$ and $A_f$, it is obtained from (S9) and (S11) for a sufficiently large $t_\epsilon \geq t_0$ that:

$$f^{\mathrm{T}} \Psi(t) + y(t) - C_0^{\mathrm{T}} z(t) - C_0^{\mathrm{T}} \Omega(t)\, \psi_a(\theta) - C_0^{\mathrm{T}} P(t)\, \psi_b(\theta) = \Gamma^{\mathrm{T}} \Psi(t)\,. \tag{S12}$$

To complete the proof that equation (9) holds, $\Psi(t)$ needs to be substituted with a known function. In order to make such substitution, the following error is introduced:

$$E(t) = \Psi(t) - F(t) + N(t)\, \psi_a(\theta) + H(t)\, \psi_b(\theta)\,. \tag{S13}$$

Equation (S13) is differentiated with respect to time:

$$\begin{array}{l} \dot{E}(t) = A_f \Psi(t) + e_n \left[y(t) - C_0^{\mathrm{T}} z(t) - C_0^{\mathrm{T}} \Omega(t)\, \psi_a(\theta) - C_0^{\mathrm{T}} P(t)\, \psi_b(\theta)\right] - \\ - A_f F(t) - e_n \left[y(t) - C_0^{\mathrm{T}} z(t)\right] + A_f N(t)\, \psi_a(\theta) + e_n C_0^{\mathrm{T}} \Omega(t)\, \psi_a(\theta) + A_f H(t)\, \psi_b(\theta) + e_n C_0^{\mathrm{T}} P(t)\, \psi_b(\theta) = \\ = A_f E(t)\,. \end{array} \tag{S14}$$

Then $E(t)$ vanishes exponentially, so for sufficiently large $t_\epsilon \geq t_0$ $\Psi(t)$ can be expressed from (S13) and substituted into (S12):

$$\left(f^{\mathrm{T}} - \Gamma^{\mathrm{T}}\right)\left[F(t) - N(t)\, \psi_a(\theta) - H(t)\, \psi_b(\theta)\right] + y(t) - C_0^{\mathrm{T}} z(t) - C_0^{\mathrm{T}} \Omega(t)\, \psi_a(\theta) - C_0^{\mathrm{T}} P(t)\, \psi_b(\theta) = 0, \tag{S15}$$

from which, considering (S9), we have that $C_0^{\mathrm{T}} \Pi(\rho)\, x_\delta(t) = \left(f^{\mathrm{T}} - \Gamma^{\mathrm{T}}\right)\left[F(t) - N(t)\, \psi_a(\theta) - H(t)\, \psi_b(\theta)\right]$.

Continuing transformations of (S15), we have:

$$\begin{array}{l} f^{\rm T}F\left(t\right)+y\left(t\right)-C_0^{\rm T}z\left(t\right)= \\ =\left(C_0^{\rm T}\Omega\left(t\right)+f^{\rm T}N\left(t\right)\right)\psi_a\left(\theta\right)+\left(C_0^{\rm T}P\left(t\right)+f^{\rm T}H\left(t\right)\right)\psi_b\left(\theta\right)+F^{\rm T}\left(t\right)\Gamma-\Gamma^{\rm T}N\left(t\right)\psi_a\left(\theta\right)-\Gamma^{\rm T}H\left(t\right)\psi_b\left(\theta\right). \end{array} \tag{S16}$$

Having vectorized equation (S16) owing to the following equalities:

$$\begin{array}{l} vec\left(\Gamma^{\rm T}N\left(t\right)\psi_a\left(\theta\right)\right)=\underbrace{\left(\psi_a^{\rm T}\left(\theta\right)\otimes\Gamma^{\rm T}\right)}_{1\times n^2}\underbrace{vec\left(N\left(t\right)\right)}_{n^2}, \\ \left[\left(\psi_a^{\rm T}\left(\theta\right)\otimes\Gamma^{\rm T}\right)vec\left(N\left(t\right)\right)\right]^{\rm T}=vec^{\rm T}\left(N\left(t\right)\right)\left(\psi_a\left(\theta\right)\otimes\Gamma\right), \\ vec\left(\Gamma^{\rm T}H\left(t\right)\psi_b\left(\theta\right)\right)=\underbrace{\left(\psi_b^{\rm T}\left(\theta\right)\otimes\Gamma^{\rm T}\right)}_{1\times n^2}\underbrace{vec\left(H\left(t\right)\right)}_{n^2}, \\ \left[\left(\psi_b^{\rm T}\left(\theta\right)\otimes\Gamma^{\rm T}\right)vec\left(H\left(t\right)\right)\right]^{\rm T}=vec^{\rm T}\left(H\left(t\right)\right)\left(\psi_b\left(\theta\right)\otimes\Gamma\right), \end{array} \tag{S17}$$

we obtain the parametrization (9).

To prove that equation (10) holds, the following set of equations is considered:

$$\begin{array}{l} \dot{e}\left(t\right)=A_Ke\left(t\right)+\psi_d\left(\theta\right)e_nh_\delta^{\rm T}x_\delta\left(t\right), \\ e_1\left(t\right)=C_0^{\rm T}e\left(t\right)=\left(\Gamma-f\right)^{\rm T}\Psi\left(t\right). \end{array} \tag{S18}$$

The output $e_1\left(t\right)$ is differentiated $n-1$ times with respect to time to obtain:

$$\begin{array}{l} e_1\left(t\right)=C_0^{\rm T}e\left(t\right), \\ \dot{e}_1\left(t\right)=C_0^{\rm T}\dot{e}\left(t\right)=C_0^{\rm T}A_Ke\left(t\right)+\psi_d\left(\theta\right)\underbrace{C_0^{\rm T}e_n}_{0}h_\delta^{\rm T}x_\delta\left(t\right), \\ \dot{e}_2\left(t\right)=C_0^{\rm T}\ddot{e}\left(t\right)=C_0^{\rm T}A_K^2e\left(t\right)+\psi_d\left(\theta\right)\underbrace{C_0^{\rm T}A_Ke_n}_{0}h_\delta^{\rm T}x_\delta\left(t\right), \\ \vdots \\ e_1^{(n-1)}\left(t\right)=C_0^{\rm T}A_K^{n-1}e\left(t\right)+\psi_d\left(\theta\right)\underbrace{C_0^{\rm T}A_K^{n-1}e_n}_{0}h_\delta^{\rm T}x_\delta\left(t\right), \end{array} \tag{S19}$$

where $C_0^{\rm T}A_K^ie_n=0$ for all $i=0,\ldots,n-2$.

For a sufficiently large $t_\epsilon\geq t_0$ equation (S19) is rewritten as follows:

$$\begin{array}{l} e_1\left(t\right)=\left(\Gamma-f\right)^{\rm T}\Psi\left(t\right), \\ \dot{e}_1\left(t\right)=\left(\Gamma-f\right)^{\rm T}A_\Gamma\Psi\left(t\right), \\ \dot{e}_2\left(t\right)=\left(\Gamma-f\right)^{\rm T}A_\Gamma^2\Psi\left(t\right), \\ \vdots \\ e_1^{(n-1)}\left(t\right)=\left(\Gamma-f\right)^{\rm T}A_\Gamma^{n-1}\Psi\left(t\right), \end{array} \tag{S20}$$

which allows one to write:

$$e\left(t\right)=\mathcal{O}_e^{-1}\mathcal{O}_\Gamma\left(\Gamma\right)\Psi\left(t\right), \tag{S21}$$

or, considering (S1) and (S13), to obtain:

$$\begin{array}{l} \xi\left(t\right)=\mathcal{O}_e^{-1}\mathcal{O}_\Gamma\left(\Gamma\right)\Psi\left(t\right)+z\left(t\right)+\Omega\left(t\right)\psi_a\left(\theta\right)+P\left(t\right)\psi_b\left(\theta\right)= \\ =\mathcal{O}_e^{-1}\mathcal{O}_\Gamma\left(\Gamma\right)\left(F\left(t\right)-N\left(t\right)\psi_a\left(\theta\right)-H\left(t\right)\psi_b\left(\theta\right)\right)+z\left(t\right)+\Omega\left(t\right)\psi_a\left(\theta\right)+P\left(t\right)\psi_b\left(\theta\right). \end{array} \tag{S22}$$

This completes proof of Proposition 1. ■

## II. Proof of Proposition 2 in the Manuscript

***Proposition 2.*** *Using procedures of extension:*

$$\begin{array}{c} q\left(t\right)=\int\limits_{t_\epsilon}^{t}e^{-\sigma\left(\tau-t_\epsilon\right)}\overline{\varphi}\left(\tau\right)\overline{q}\left(\tau\right)d\tau, \\ \varphi\left(t\right)=\int\limits_{t_\epsilon}^{t}e^{-\sigma\left(\tau-t_\epsilon\right)}\overline{\varphi}\left(\tau\right)\overline{\varphi}^{\rm T}\left(\tau\right)d\tau, \\ q\left(t_\epsilon\right)=0_{2n},\ \varphi\left(t_\epsilon\right)=0_{2n\times2n}, \end{array} \tag{16}$$

*and mixing:*

$$\begin{array}{c} \mathcal{Y}\left(t\right)=k\left(t\right)\cdot{\rm adj}\left\{\varphi\left(t\right)\right\}q\left(t\right), \\ \Delta\left(t\right)=k\left(t\right)\cdot\det\left\{\varphi\left(t\right)\right\}, \end{array} \tag{17}$$

*for all $t \geq t_\epsilon$ a set of scalar regression equations is obtained:*

$$\mathcal{Y}(t) = \Delta(t)\,\eta(\psi), \tag{18}$$

*where $\sigma > 0$ is a damping factor, $k(t) \geq k_{\min} > 0$ is an amplitude amplifier and for all $t \geq t_e$ it holds that $\Delta(t) \geq$ $\geq \Delta_{\min} > 0$ when $\overline{\varphi} \in$ FE over $[t_\epsilon,\, t_e]$.*

*Proof:*

The function $\overline{q}(t)$ from (13) is substituted into the differential equation for $q(t)$ from (16):

$$\dot{q}(t) = e^{-\sigma(t-t_\epsilon)}\overline{\varphi}(t)\,\overline{q}(t) = e^{-\sigma(t-t_\epsilon)}\overline{\varphi}(t)\,\overline{\varphi}^{\mathrm{T}}(t)\,\eta(\theta) = \dot{\varphi}(t)\,\eta(\psi), \tag{S23}$$

then the solution of (S23) is substituted into $k(t)\cdot \mathrm{adj}\{\varphi(t)\}\,q(t)$ to obtain (18):

$$k(t)\cdot \mathrm{adj}\{\varphi(t)\}\,q(t) = k(t)\cdot \mathrm{adj}\{\varphi(t)\}\,\varphi(t)\,\eta(\psi) = \Delta(t)\,\eta(\psi) = \mathcal{Y}(t). \tag{S24}$$

If $\overline{\varphi} \in$ FE over $[t_\epsilon,\, t_e]$, then for all $t \geq t_\epsilon$ equation (2) holds, therefore, the following can be written:

$$\begin{gathered}\Delta(t) = k(t)\cdot \det\{\varphi(t)\} = k(t)\cdot \det\left\{\int\limits_{t_\epsilon}^{t} e^{-\sigma(\tau-t_\epsilon)}\overline{\varphi}(\tau)\,\overline{\varphi}^{\mathrm{T}}(\tau)\,d\tau\right\} \geq \\ \geq k(t)\cdot \det\left\{\int\limits_{t_\epsilon}^{t_e} e^{-\sigma(\tau-t_\epsilon)}\overline{\varphi}(\tau)\,\overline{\varphi}^{\mathrm{T}}(\tau)\,d\tau\right\} \geq k_{\min}\det\left\{\alpha e^{-\sigma(t_e-t_\epsilon)}I_n\right\} > 0,\end{gathered} \tag{S25}$$

from which it follows that $\Delta(t) \geq \Delta_{\min} = k_{\min}\det\left\{\alpha e^{-\sigma(t_e-t_\epsilon)}I_n\right\} > 0$ for all $t \geq t_e$.

■

## III. Proof of Lemma in the Manuscript

***Lemma.*** *For all $t \geq t_\epsilon$ the unknown parameters $\kappa = \begin{bmatrix}\psi^{\mathrm{T}} & vec^{\mathrm{T}}(\mathcal{O}_\Gamma(\Gamma)) & vec^{\mathrm{T}}(T_I(\theta))\end{bmatrix}^{\mathrm{T}}$ satisfy the following regression equation:*

$$\begin{gathered}\mathcal{Y}_\kappa(t) = \mathcal{M}_\kappa(t)\,\kappa, \\ \mathcal{Y}_\kappa(t) = \mathrm{adj}\{\mathrm{bd}\{\mathcal{M}_\psi(t),\, \mathcal{M}_{\mathcal{O}_\Gamma}(t),\, \mathcal{M}_{T_I}(t)\}\}\begin{bmatrix}\mathcal{Y}_\psi(t) \\ vec(\mathcal{Y}_{\mathcal{O}_\Gamma}(t)) \\ vec(\mathcal{Y}_{T_I}(t))\end{bmatrix}, \\ \mathcal{M}_\kappa(t) = \det\{\mathrm{bd}\{\mathcal{M}_\psi I_{3n},\, \mathcal{M}_{\mathcal{O}_\Gamma} I_{n^2},\, \mathcal{M}_{T_I} I_{n^2}\}\}\end{gathered} \tag{25}$$

*where:*

*1) the regressand and regressor of $\mathcal{Y}_\psi(t) = \mathcal{M}_\psi(t)\,\psi$ are defined as follows:*

$$\begin{gathered}\mathcal{Y}_\psi(t) = \mathrm{adj}\left\{\mathcal{T}_{\mathcal{G}_\psi}\left(\Xi_{\mathcal{G}_\psi}(\Delta)\,\mathcal{Y}\right)\right\}\mathcal{T}_{\mathcal{S}_\psi}\left(\Xi_{\mathcal{S}_\psi}(\Delta)\,\mathcal{Y}\right), \\ \mathcal{M}_\psi(t) = \det\left\{\mathcal{T}_{\mathcal{G}_\psi}\left(\Xi_{\mathcal{G}_\psi}(\Delta)\,\mathcal{Y}\right)\right\},\end{gathered}$$

*2) the regressand and regressor of $\mathcal{Y}_{\mathcal{O}_\Gamma}(t) = \mathcal{M}_{\mathcal{O}_\Gamma}(t)\,\mathcal{O}_\Gamma(\Gamma)$ are defined as follows:*

$$\begin{gathered}\mathcal{Y}_{\mathcal{O}_\Gamma}(t) = \mathrm{adj}\{\Pi_{\mathcal{O}_\Gamma}(\mathcal{M}_\psi)\}\,\mathcal{T}_{\mathcal{O}_\Gamma}\left(\Xi_{\mathcal{O}_\Gamma}(\mathcal{M}_\psi)\,\mathcal{Y}_\Gamma\right), \\ \mathcal{M}_{\mathcal{O}_\Gamma}(t) = \det\{\Pi_{\mathcal{O}}(\mathcal{M}_\psi)\},\end{gathered}$$

*where $\mathcal{Y}_\Gamma(t) = \mathcal{L}_\Gamma\mathcal{Y}_\psi(t)$, and $\mathcal{L}_\Gamma$ is such that $\mathcal{L}_\Gamma\psi = \Gamma$.*

*3) the regressand and regressor of $\mathcal{Y}_{T_I}(t) = \mathcal{M}_{T_I}(t)\,T_I(\theta)$, considering auxiliary equations:*

$$\begin{gathered}\mathcal{Y}_\theta(t) = \mathrm{adj}\left\{\mathcal{T}_{\mathcal{G}_\theta}\left(\Xi_{\mathcal{G}_\theta}(\mathcal{M}_\psi)\,\mathcal{Y}_{ab}\right)\right\}\mathcal{T}_{\mathcal{S}_\theta}\left(\Xi_{\mathcal{S}_\theta}(\mathcal{M}_\psi)\,\mathcal{Y}_{ab}\right), \\ \mathcal{M}_\theta(t) = \det\left\{\mathcal{T}_{\mathcal{G}_\theta}\left(\Xi_{\mathcal{G}_\theta}(\mathcal{M}_\psi)\,\mathcal{Y}_{ab}\right)\right\},\end{gathered}$$

*are defined as follows:*

$$\begin{gathered}\mathcal{Y}_{T_I}(t) = \mathrm{adj}\left\{\mathcal{T}_{\mathcal{P}}\left(\Xi_{\mathcal{P}}(\mathcal{M}_\theta)\,\mathcal{Y}_\theta\right)\right\}\mathcal{T}_{\mathcal{Q}}\left(\Xi_{\mathcal{Q}}(\mathcal{M}_\theta)\,\mathcal{Y}_\theta\right), \\ \mathcal{M}_{T_I}(t) = \det\left\{\mathcal{T}_{\mathcal{P}}\left(\Xi_{\mathcal{P}}(\mathcal{M}_\theta)\,\mathcal{Y}_\theta\right)\right\},\end{gathered}$$

*where $\mathcal{Y}_{ab}(t) = \mathcal{L}_{ab}\mathcal{Y}_\psi(t)$, and $\mathcal{L}_{ab}$ is defined in (14).*

*If additionally $\overline{\varphi} \in$ FE over $[t_\epsilon,\, t_e]$, then for all $t \geq t_e$ the inequality $|\mathcal{M}_\kappa(t)| \geq \underline{\mathcal{M}_\kappa} > 0$ holds.*

*Proof:*

In accordance with Definition 1 and Hypothesis 2 and owing to:

$$\begin{gathered}\Xi_{\mathcal{S}_\psi}(\Delta) = \overline{\Xi}_{\mathcal{S}_\psi}(\Delta)\,\Delta(t), \\ \Xi_{\mathcal{G}_\psi}(\Delta) = \overline{\Xi}_{\mathcal{G}_\psi}(\Delta)\,\Delta(t), \\ \overline{\Xi}_{\mathcal{S}_\psi}(\Delta)\,\Delta(t)\,\eta(\psi) = \Xi_{\mathcal{S}_\psi}(\Delta)\,\mathcal{Y}(t), \\ \overline{\Xi}_{\mathcal{G}_\psi}(\Delta)\,\Delta(t)\,\eta(\psi) = \overline{\Xi}_{\mathcal{G}_\psi}\mathcal{Y}(t),\end{gathered}$$

the following equality is obtained from (21):

$$\mathcal{T}_{\mathcal{S}_\psi}\left(\overline{\Xi}_{\mathcal{S}_\psi}(\Delta)\mathcal{Y}\right)=\mathcal{T}_{\mathcal{G}_\psi}\left(\overline{\Xi}_{\mathcal{G}_\psi}(\Delta)\mathcal{Y}\right)\psi. \tag{S26}$$

Then, having multiplied (S26) by $\operatorname{adj}\left\{\mathcal{T}_{\mathcal{G}_\psi}\left(\overline{\Xi}_{\mathcal{G}_\psi}(\Delta)\mathcal{Y}\right)\right\}$, the following regression equation is obtained:

$$\begin{gathered}\mathcal{Y}_\psi(t)=\operatorname{adj}\left\{\mathcal{T}_{\mathcal{G}_\psi}\left(\overline{\Xi}_{\mathcal{G}_\psi}(\Delta)\mathcal{Y}\right)\right\}\mathcal{T}_{\mathcal{S}_\psi}\left(\overline{\Xi}_{\mathcal{S}_\psi}(\Delta)\mathcal{Y}\right)=\mathcal{M}_\psi(t)\psi,\\ \mathcal{M}_\psi(t)=\det\left\{\mathcal{T}_{\mathcal{G}_\psi}\left(\overline{\Xi}_{\mathcal{G}_\psi}(\Delta)\mathcal{Y}\right)\right\},\end{gathered} \tag{S27}$$

using which together with (24) and owing to:

$$\Xi_{\mathcal{O}_\Gamma}(\mathcal{M}_\psi)\Gamma=\overline{\Xi}_{\mathcal{O}_\Gamma}(\mathcal{M}_\psi)\mathcal{M}_\psi(t)\Gamma=\overline{\Xi}_{\mathcal{O}_\Gamma}(\mathcal{M}_\psi)\mathcal{Y}_\Gamma(t),$$

it is obtained that:

$$\mathcal{T}_{\mathcal{O}_\Gamma}\left(\overline{\Xi}_{\mathcal{O}_\Gamma}(\mathcal{M}_\psi)\mathcal{Y}_\Gamma\right)=\Pi_{\mathcal{O}_\Gamma}(\mathcal{M}_\psi)\mathcal{O}_\Gamma(\Gamma). \tag{S28}$$

Having multiplied (S28) by $\operatorname{adj}\{\Pi_{\mathcal{O}_\Gamma}(\mathcal{M}_\psi)\}$, the following regression equation is obtained:

$$\begin{gathered}\mathcal{Y}_{\mathcal{O}_\Gamma}(t)=\operatorname{adj}\{\Pi_{\mathcal{O}_\Gamma}(\mathcal{M}_\psi)\}\mathcal{T}_{\mathcal{O}_\Gamma}\left(\overline{\Xi}_{\mathcal{O}_\Gamma}(\mathcal{M}_\psi)\mathcal{Y}_\Gamma\right)=\mathcal{M}_{\mathcal{O}_\Gamma}(t)\mathcal{O}_\Gamma(\Gamma),\\ \mathcal{M}_{\mathcal{O}_\Gamma}(t)=\det\{\Pi_{\mathcal{O}}(\mathcal{M}_\psi)\}.\end{gathered} \tag{S29}$$

Following Definition 1 and Hypothesis 2 and owing to:

$$\begin{gathered}\Xi_{\mathcal{S}_\theta}(\mathcal{M}_\psi)=\overline{\Xi}_{\mathcal{S}_\theta}(\mathcal{M}_\psi)\mathcal{M}_\psi(t),\\ \Xi_{\mathcal{G}_\theta}(\mathcal{M}_\psi)=\overline{\Xi}_{\mathcal{G}_\theta}(\mathcal{M}_\psi)\mathcal{M}_\psi(t),\\ \overline{\Xi}_{\mathcal{S}_\theta}(\mathcal{M}_\psi)\mathcal{M}_\psi(t)\psi_{ab}(\theta)=\overline{\Xi}_{\mathcal{S}_\psi}(\mathcal{M}_\psi)\mathcal{Y}_{ab}(t),\\ \overline{\Xi}_{\mathcal{G}_\theta}(\Delta)\mathcal{M}_\psi(t)\psi_{ab}(\theta)=\overline{\Xi}_{\mathcal{G}_\psi}(\mathcal{M}_\psi)\mathcal{Y}_{ab}(t),\end{gathered}$$

the following equality is obtained from (22):

$$\mathcal{T}_{\mathcal{S}_\theta}\left(\overline{\Xi}_{\mathcal{S}_\theta}(\mathcal{M}_\psi)\mathcal{Y}_{ab}\right)=\mathcal{T}_{\mathcal{G}_\theta}\left(\overline{\Xi}_{\mathcal{G}_\theta}(\mathcal{M}_\psi)\mathcal{Y}_{ab}\right)\theta. \tag{S30}$$

Then, having multiplied (S30) by $\operatorname{adj}\left\{\mathcal{T}_{\mathcal{G}_\theta}\left(\overline{\Xi}_{\mathcal{G}_\theta}(\mathcal{M}_\psi)\mathcal{Y}_{ab}\right)\right\}$, the following regression equation is obtained:

$$\begin{gathered}\mathcal{Y}_\theta(t)=\operatorname{adj}\left\{\mathcal{T}_{\mathcal{G}_\theta}\left(\overline{\Xi}_{\mathcal{G}_\theta}(\mathcal{M}_\psi)\mathcal{Y}_{ab}\right)\right\}\mathcal{T}_{\mathcal{S}_\theta}\left(\overline{\Xi}_{\mathcal{S}_\theta}(\mathcal{M}_\psi)\mathcal{Y}_{ab}\right)=\mathcal{M}_\theta(t)\theta,\\ \mathcal{M}_\theta(t)=\det\left\{\mathcal{T}_{\mathcal{G}_\theta}\left(\overline{\Xi}_{\mathcal{G}_\theta}(\mathcal{M}_\psi)\mathcal{Y}_{ab}\right)\right\},\end{gathered} \tag{S31}$$

using which together with (23) and owing to:

$$\begin{gathered}\Xi_{\mathcal{P}}(\mathcal{M}_\theta)=\overline{\Xi}_{\mathcal{P}}(\mathcal{M}_\theta)\mathcal{M}_\theta(t),\\ \Xi_{\mathcal{Q}}(\mathcal{M}_\theta)=\overline{\Xi}_{\mathcal{Q}}(\mathcal{M}_\theta)\mathcal{M}_\theta(t),\\ \overline{\Xi}_{\mathcal{P}}(\mathcal{M}_\theta)\mathcal{M}_\theta(t)\theta=\overline{\Xi}_{\mathcal{P}}(\mathcal{M}_\theta)\mathcal{Y}_\theta(t),\\ \overline{\Xi}_{\mathcal{Q}}(\mathcal{M}_\theta)\mathcal{M}_\theta(t)\theta=\overline{\Xi}_{\mathcal{Q}}(\mathcal{M}_\theta)\mathcal{Y}_\theta(t),\end{gathered}$$

it is obtained that:

$$\mathcal{T}_{\mathcal{Q}}\left(\overline{\Xi}_{\mathcal{Q}}(\mathcal{M}_\theta)\mathcal{Y}_\theta\right)=\mathcal{T}_{\mathcal{P}}\left(\overline{\Xi}_{\mathcal{P}}(\mathcal{M}_\theta)\mathcal{Y}_\theta\right)T_I(\theta). \tag{S32}$$

Having multiplied (S32) by $\operatorname{adj}\left\{\mathcal{T}_{\mathcal{P}}\left(\overline{\Xi}_{\mathcal{P}}(\mathcal{M}_\theta)\mathcal{Y}_\theta\right)\right\}$, the following regression equation is obtained:

$$\begin{gathered}\mathcal{Y}_{T_I}(t)=\operatorname{adj}\left\{\mathcal{T}_{\mathcal{P}}\left(\overline{\Xi}_{\mathcal{P}}(\mathcal{M}_\theta)\mathcal{Y}_\theta\right)\right\}\mathcal{T}_{\mathcal{Q}}\left(\overline{\Xi}_{\mathcal{Q}}(\mathcal{M}_\theta)\mathcal{Y}_\theta\right)=\mathcal{M}_{T_I}(t)T_I(\theta),\\ \mathcal{M}_{T_I}(t)=\det\left\{\mathcal{T}_{\mathcal{P}}\left(\overline{\Xi}_{\mathcal{P}}(\mathcal{M}_\theta)\mathcal{Y}_\theta\right)\right\}.\end{gathered} \tag{S33}$$

Using proved claims from Proposition 2, if $\overline{\varphi}\in\text{FE}$, then for all $t\geq t_e$ it is true that $\Delta(t)\geq\Delta_{\min}>0$, and, according to Hypothesis 2, it holds that:

$$\begin{gathered}\det{}^2\{\mathcal{G}_\psi(\eta)\}>0,\ \det{}^2\{\mathcal{G}_\theta(\psi_{ab})\}>0,\ \det{}^2\{\mathcal{P}(\theta)\}>0,\\ \det\{\mathcal{I}\}\geq\arg\{\mathcal{I}\}^{\ell_{\mathcal{I}}},\mathcal{I}\in\{\Pi_\psi(\Delta),\Pi_\theta(\mathcal{M}_\psi),\Pi_{T_I}(\mathcal{M}_\theta),\Pi_{\mathcal{O}_\Gamma}(\mathcal{M}_\psi)\},\end{gathered}$$

from which for all $t\geq t_e$ the following inequalities hold if $\overline{\varphi}\in\text{FE}$:

$$\begin{array}{l}|\mathcal{M}_\psi(t)|=|\det\{\Pi_\psi(\Delta)\mathcal{G}_\psi(\eta)\}|=|\det\{\Pi_\psi(\Delta)\}\det\{\mathcal{G}_\psi(\eta)\}|\geq\\ \geq\left|\Delta^{\ell_\psi}(t)\det\{\mathcal{G}_\psi(\eta)\}\right|\geq\Delta_{\min}^{\ell_\psi}|\det\{\mathcal{G}_\psi(\eta)\}|=\underline{\mathcal{M}}_\psi>0,\\ |\mathcal{M}_{\mathcal{O}_\Gamma}(t)|=|\det\{\Pi_{\mathcal{O}_\Gamma}(\mathcal{M}_\psi)\}|\geq\underline{\mathcal{M}}_\psi^{\ell_{\mathcal{O}_\Gamma}}=\underline{\mathcal{M}}_{\mathcal{O}_\Gamma}>0,\\ |\mathcal{M}_\theta(t)|=|\det\{\Pi_\theta(\mathcal{M}_\psi)\mathcal{G}_\theta(\psi_{ab})\}|=|\det\{\Pi_\theta(\mathcal{M}_\psi)\}\det\{\mathcal{G}_\theta(\psi_{ab})\}|\geq\\ \geq\left|\mathcal{M}_\psi^{\ell_\theta}(t)\det\{\mathcal{G}_\theta(\psi_{ab})\}\right|\geq\underline{\mathcal{M}}_\psi^{\ell_\theta}|\det\{\mathcal{G}_\theta(\psi_{ab})\}|=\underline{\mathcal{M}}_\theta>0,\\ |\mathcal{M}_{T_I}(t)|=|\det\{\Pi_{T_I}(\mathcal{M}_\theta)\mathcal{P}(\theta)\}|=|\det\{\Pi_{T_I}(\mathcal{M}_\theta)\}\det\{\mathcal{P}(\theta)\}|\geq\\ \geq\left|\mathcal{M}_\theta^{\ell_{T_I}}(t)\det\{\mathcal{P}(\theta)\}\right|\geq\underline{\mathcal{M}}_\theta^{\ell_{T_I}}|\det\{\mathcal{P}(\theta)\}|=\underline{\mathcal{M}}_{T_I}>0,\end{array} \tag{S34}$$

which allows one to write:

$$\left|\mathcal{M}_{\kappa}(t)\right| = \left|\mathcal{M}_{\psi}^{3n}(t)\,\mathcal{M}_{\mathcal{O}_{\Gamma}}^{n^2}(t)\,\mathcal{M}_{T_I}^{n^2}(t)\right| \geq \underline{\mathcal{M}}_{\psi}^{3n}\underline{\mathcal{M}}_{\mathcal{O}_{\Gamma}}^{n^2}\underline{\mathcal{M}}_{T_I}^{n^2} = \underline{\mathcal{M}}_{\kappa} > 0. \tag{S35}$$

■

## IV. Derivation of the equation (27) in the Manuscript

Equation (27) is obtained in the following way:

$$\begin{array}{l}
\tilde{x}(t) = \hat{T}_I(t)\,\hat{\xi}(t) - T_I(\theta)\,\xi(t) \pm T_I(\theta)\,\hat{\xi}(t) = \tilde{T}_I(t)\,\hat{\xi}(t) + T_I(\theta)\,\tilde{\xi}(t) \pm \tilde{T}_I(\theta)\,\xi(t) = \\
= \tilde{T}_I(t)\,\tilde{\xi}(t) + T_I(\theta)\,\tilde{\xi}(t) + \tilde{T}_I(t)\,\xi(t)\,, \\
\tilde{\xi}(t) = \mathcal{O}_e^{-1}\hat{\mathcal{O}}_{\Gamma}(t)\left(F(t) - N(t)\,\hat{\psi}_a(t) - H(t)\,\hat{\psi}_b(t)\right) + z(t) + \Omega(t)\,\hat{\psi}_a(t) + P(t)\,\hat{\psi}_b(t) - \\
-\mathcal{O}_e^{-1}\mathcal{O}_{\Gamma}(\Gamma)\left(F(t) - N(t)\,\psi_a(\theta) - H(t)\,\psi_b(\theta)\right) - z(t) - \Omega(t)\,\psi_a(\theta) - P(t)\,\psi_b(\theta) = \\
= \mathcal{O}_e^{-1}\hat{\mathcal{O}}_{\Gamma}(t)\left(F(t) - N(t)\,\hat{\psi}_a(t) - H(t)\,\hat{\psi}_b(t)\right) - \mathcal{O}_e^{-1}\mathcal{O}_{\Gamma}(\Gamma)\left(F(t) - N(t)\,\psi_a(\theta) - H(t)\,\psi_b(\theta)\right) + \\
+\Omega(t)\,\tilde{\psi}_a(t) + P(t)\,\tilde{\psi}_b(t) \pm \mathcal{O}_e^{-1}\hat{\mathcal{O}}_{\Gamma}(t)\left(F(t) - N(t)\,\psi_a(\theta) - H(t)\,\psi_b(\theta)\right) = \\
= \mathcal{O}_e^{-1}\hat{\mathcal{O}}_{\Gamma}(t)\left(-N(t)\,\tilde{\psi}_a(t) - H(t)\,\tilde{\psi}_b(t)\right) + \mathcal{O}_e^{-1}\tilde{\mathcal{O}}_{\Gamma}(t)\left(F(t) - N(t)\,\psi_a(\theta) - H(t)\,\psi_b(\theta)\right) + \\
+\Omega(t)\,\tilde{\psi}_a(t) + P(t)\,\tilde{\psi}_b(t) \pm \mathcal{O}_e^{-1}\mathcal{O}_{\Gamma}(\Gamma)\left(-N(t)\,\tilde{\psi}_a(t) - H(t)\,\tilde{\psi}_b(t)\right) = \\
= \mathcal{O}_e^{-1}\tilde{\mathcal{O}}_{\Gamma}(t)\left(-N(t)\,\tilde{\psi}_a(t) - H(t)\,\tilde{\psi}_b(t)\right) + \mathcal{O}_e^{-1}\tilde{\mathcal{O}}_{\Gamma}(t)\left(F(t) - N(t)\,\psi_a(\theta) - H(t)\,\psi_b(\theta)\right) + \\
+\Omega(t)\,\tilde{\psi}_a(t) + P(t)\,\tilde{\psi}_b(t) + \mathcal{O}_e^{-1}\mathcal{O}_{\Gamma}(\Gamma)\left(-N(t)\,\tilde{\psi}_a(t) - H(t)\,\tilde{\psi}_b(t)\right).
\end{array} \tag{S36}$$

## V. Derivation of the equation (35) in the Manuscript

***Derivation of (35).*** The bellow-given equalities follow from definition of $\eta(\psi)$:

$$\begin{array}{l}
\eta_1 = \psi_{a2} + \rho, \\
\eta_2 = \psi_{b1}, \\
\eta_3 = \psi_{b3} - \psi_{b1}\rho, \\
\eta_4 = -\psi_{a2}\rho, \\
\eta_5 = -\psi_{b3}\rho.
\end{array} \tag{S37}$$

The component $\eta_4$ is divided by $\eta_5$, and $\psi_{a2}$ is expressed from the obtained result:

$$\begin{array}{l}
\frac{\eta_4}{\eta_5} = \frac{\psi_{a2}}{\psi_{b3}}, \\
\psi_{a2} = \frac{\eta_4}{\eta_5}\psi_{b3}.
\end{array} \tag{S38}$$

Equation (S38) is substituted into expression for $\eta_1$, and $\psi_{b3}$ is expressed from the obtained result:

$$\begin{array}{l}
\eta_1 = \psi_{a2} + \rho = \frac{\eta_4}{\eta_5}\psi_{b3} + \rho, \\
\psi_{b3} = (\eta_1 - \rho)\,\frac{\eta_5}{\eta_4}.
\end{array} \tag{S39}$$

Taking into consideration the equality $\eta_2 = \psi_{b1}$, equation (S39) is substituted into the expression for $\eta_3$:

$$\eta_3 = \psi_{b3} - \psi_{b1}\rho = \psi_{b3} - \eta_2\rho = (\eta_1 - \rho)\,\frac{\eta_5}{\eta_4} - \eta_2\rho, \tag{S40}$$

from which we have:

$$\begin{array}{l}
\eta_3 - \eta_1\frac{\eta_5}{\eta_4} = -\left(\frac{\eta_5}{\eta_4} + \eta_2\right)\rho, \\
\rho = \frac{\eta_4\eta_3 - \eta_1\eta_5}{-(\eta_5 + \eta_4\eta_2)},
\end{array} \tag{S41}$$

which, in its turn, allows one to write:

$$\psi_{a2} = \eta_1 + \frac{\eta_4\eta_3 - \eta_1\eta_5}{\eta_5 + \eta_4\eta_2}, \tag{S42}$$

$$\psi_{b3} = \frac{\eta_5(\eta_5 + \eta_4\eta_2)}{\eta_4\eta_3 - \eta_1\eta_5}. \tag{S43}$$

Introducing the respective change of notation, equation (35) is obtained.

## VI. Verification of Hypothesis 1.

The following linear system is considered:

$$\begin{aligned} &\dot{x}(t) = \theta_1 x(t) + \theta_2 u(t) + \delta(t), \\ &\dot{x}_\delta(t) = \begin{bmatrix} 0 & 1 \\ \rho & 0 \end{bmatrix} x_\delta(t),\; x_\delta(t_0) = x_{\delta 0}, \\ &\delta(t) = \begin{bmatrix} 1 & 0 \end{bmatrix} x_\delta(t). \end{aligned} \tag{S44}$$

The parameters of (S44) and filters (12) are set as follows:

$$\theta_1 = -0.25,\; \theta_2 = 5.65,\; x_\delta(t_0) = \begin{bmatrix} 1 & 2 \end{bmatrix}^{\mathrm{T}},\, \rho = -10,\; K = 5,\; f = -1. \tag{S45}$$

The control signal $u(t)$ is chosen as:

$$u(t) = \sin(0.1\mathrm{t}) + 2.5\sin(1\mathrm{t}) + 10\sin(10t). \tag{S46}$$

Figure S1 presents the behavior of the elements of the regressor $\overline{\varphi}_e(t)$.

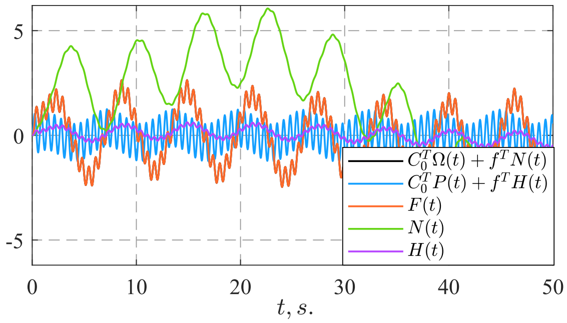


Fig. S1. Behavior of regressor $\overline{\varphi}_e(t)$ elements.

As it follows from Fig. S1, it holds that $F(t) = \Omega^{\mathrm{T}}(t)\,C_0 + N^{\mathrm{T}}(t)\,f$. So regressor $\overline{\varphi}_e(t)$ can not satisfy the finite excitation condition (2). Let us demonstrate that in case $n = 1$ such equality holds independently from the values of the parameters of the system (S44), filters (12) and control signal. To do that, the following error is introduced:

$$\varepsilon(t) = F(t) - \Omega^{\mathrm{T}}(t)\,C_0 - N^{\mathrm{T}}(t)\,f,\, \varepsilon(t_0) = 0. \tag{S47}$$

Equation (S47) is differentiated with respect to time to obtain:

$$\begin{aligned} &\dot{\varepsilon}(t) = A_f F + e_n\left[y - C_0^{\mathrm{T}} z\right] - \left(\Omega^{\mathrm{T}} A_K^{\mathrm{T}} + I_n y\right) C_0 - \left(N^{\mathrm{T}} A_f^{\mathrm{T}} + \Omega^{\mathrm{T}} C_0 e_n^{\mathrm{T}}\right) f = \\ &= e_n^{\mathrm{T}} f\left[F - \Omega^{\mathrm{T}} C_0 - N^{\mathrm{T}} f\right] + N^{\mathrm{T}}\left(f e_n^{\mathrm{T}} f - A_f^{\mathrm{T}} f\right) + \left(A_f - e_n^{\mathrm{T}} f\right) F + \\ &+ e_n\left[y - C_0^{\mathrm{T}} z\right] - y I_n C_0 - \Omega^{\mathrm{T}} A_K^{\mathrm{T}} C_0 = \\ &= e_n^{\mathrm{T}} f \varepsilon(t) + N^{\mathrm{T}}\left(f e_n^{\mathrm{T}} f - A_f^{\mathrm{T}} f\right) + \left(A_f - e_n^{\mathrm{T}} f\right) F + e_n\left[y - C_0^{\mathrm{T}} z\right] - y I_n C_0 - \Omega^{\mathrm{T}} A_K^{\mathrm{T}} C_0. \end{aligned} \tag{S48}$$

In case under consideration we have:

$$e_1^{\mathrm{T}} = 1,\; A_f = f,\, C_0 = 1,\; I_1 = 1,\; A_K^{\mathrm{T}} = -K,\, \Omega^{\mathrm{T}}(t) = \Omega(t), \tag{S49}$$

which allows one to rewrite (S48) in the following form:

$$\dot{\varepsilon}(t) = f\varepsilon(t) + K\Omega(t) - z(t). \tag{S50}$$

The following error is considered:

$$\varepsilon_1(t) = K\Omega(t) - z(t),\, \varepsilon_1(t_0) = 0. \tag{S51}$$

Equation (S51) is differentiated with respect to time and, considering (S49), it is written:

$$\dot{\varepsilon}_1(t) = K\left[A_K \Omega(t) + I_n y(t)\right] - \left[A_K z(t) + K y(t)\right] = -K\left[K\Omega(t) - z(t)\right] = -K\varepsilon_1(t). \tag{S52}$$

As $\varepsilon_1(t_0) = 0$, then $\varepsilon_1(t) = 0\;\forall t \geq t_0$, and since $\varepsilon(t_0) = 0$, then $\varepsilon(t) = 0\;\forall t \geq t_0$, so in case $n = 1$ the equality $F(t) = \Omega^{\mathrm{T}}(t)\,C_0 + N^{\mathrm{T}}(t)\,f$ holds independently from the control signal, as well as from the parameters of the system (S44) and filters (12). So for the case $n = 1$ and $n_\delta = 2$ there always exists $i = 1$ and $j = 3$ such that $e_1^{\mathrm{T}}\overline{\varphi}_e(t) = e_3^{\mathrm{T}}\overline{\varphi}_e(t)$, and consequently Hypothesis 1 is verified.

Unfortunately, at the moment for generalized case $n \geq 1$ and $n_\delta \geq 2$ we cannot provide a theoretically sound proof that there always exists $i \neq j$ such that $e_i^{\rm T}\overline{\varphi}_e\left(t\right) = e_j^{\rm T}\overline{\varphi}_e\left(t\right)$. However, in the many simulation examples this is the case, e.g. for the plant (29) we have that $e_2^{\rm T}\overline{\varphi}_e\left(t\right) = e_8^{\rm T}\overline{\varphi}_e\left(t\right),\, e_6^{\rm T}\overline{\varphi}_e\left(t\right) = e_{20}^{\rm T}\overline{\varphi}_e\left(t\right)$ for all control inputs, all system and filters (12) parameters. Therefore, in order to implement the proposed observer, we now need some preliminary simulations to find indices of equal elements of the regressor $\overline{\varphi}_e\left(t\right)$, which are required to find eliminators from Hypothesis 1.

## VII. Reference to example that demonstrates that assumptions/hypotheses are not restrictive

For an example that demonstrates that assumptions/hypotheses are not restrictive please see section VI of [S1].

## References

[S1] Glushchenko A., Lastochkin K. "Adaptive Observer of State and Disturbances for Linear Overparameterized Systems", *Automation and Remote Control*, 2023, Vol.84, No.11, pp.1208-1231.
